# Supplementary material for: Live Laparoscopic Video Retrieval with Compressed Uncertainty
Source: arXiv:2203.04301 ancillary file (2023-06-12)
Supplement: Supplementary file 1 [file supplementary_material.pdf]

## A - List of surgical phases

### Cholec80

| CHOLEC 80                 |                                                                                        |                                                                                       |                |
|---------------------------|----------------------------------------------------------------------------------------|---------------------------------------------------------------------------------------|----------------|
| Name                      | Description                                                                            |                                                                                       | Duration (min) |
| Preparation               | Exposure of gallbladder by removal of surrounding tissue                               | 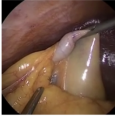   | 1.8±1.7        |
| Calot triangle dissection | Exposure of the base of the liver bed by dissecting the neck of the gallbladder        | 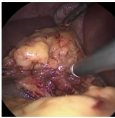   | 15.6±11.1      |
| Clipping & cutting        | Application of clips to the cystic duct, cutting of cystic duct                        | 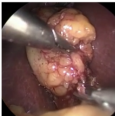   | 2.9±2.1        |
| Gallbladder dissection    | Dissection of gallbladder from the liver bed                                           | 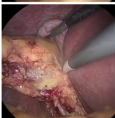   | 12.2±8.9       |
| Gallbladder packaging     | Insertion of dissected gallbladder into specimen bag                                   | 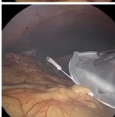  | 1.6±0.8        |
| Cleaning & coagulation    | Coagulation of the liver bed and cleanup using the irrigation & suction device         | 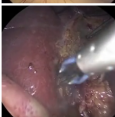 | 3.0±2.6        |
| Gallbladder extraction    | Extraction of the specimen bag containing the gallbladder through the umbilical trocar | 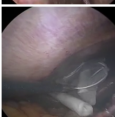 | 1.4±1.2        |

Figure 1: Phase breakdown of cholecystectomy in the Cholec80 dataset

## Bypass40

| BYPASS 40                    |                                                                                                                  |                                                                                       |                |
|------------------------------|------------------------------------------------------------------------------------------------------------------|---------------------------------------------------------------------------------------|----------------|
| Name                         | Description                                                                                                      |                                                                                       | Duration (min) |
| Preparation                  | Access to abdominal cavity, installation of ports for the instruments & the camera, exposure of operating field  | 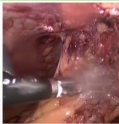   | $7.1 \pm 2.9$  |
| Gastric pouch creation       | Isolation of the part of the stomach adjacent to the oesophagus, to create a reduced gastric pouch               | 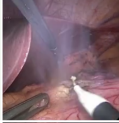   | $25.6 \pm 8.1$ |
| Omentum division             | Vertical section of the omentum to facilitate the ascent of the small intestine to the gastric pouch             | 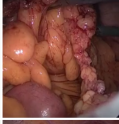   | $23.1 \pm 5.5$ |
| Gastrojejunal anastomosis    | Connection of the distal small intestine with the gastric pouch                                                  | 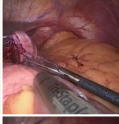   | $3.3 \pm 0.6$  |
| Anastomosis test             | Leak control of gastrojejunostomy                                                                                | 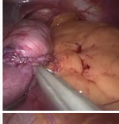  | $2.8 \pm 0.8$  |
| Jejunal separation           | Separation between biliary and alimentary limb                                                                   | 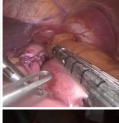 | $3.1 \pm 0.6$  |
| Closure of Petersen space    | Closure of space created between the mesentery and the mesocolon as the small intestine rises to make the bypass | 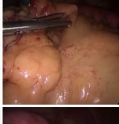 | $7.4 \pm 2.2$  |
| Jejunojejunal anastomosis    | Connection of the biliary limb with the alimentary limb                                                          | 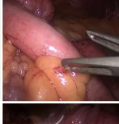 | $23.9 \pm 7.6$ |
| Closure of mesenteric defect | Closure of the space created in the mesentery as the small intestine rises to make the bypass                    | 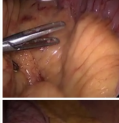 | $9.2 \pm 2.1$  |
| Cleaning and coagulation     | Verification of absence of bleeding; hemostasis and aspiration of remaining fluids in the abdominal cavity       | 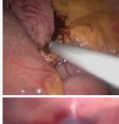 | $4.2 \pm 1.0$  |
| Disassembling                | Removal of surgical instruments, ports and camera                                                                | 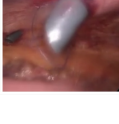 | $5.9 \pm 1.4$  |

Figure 2: Phase breakdown of gastric bypass in the Bypass40 dataset

## B - Additional results for ULA-CODE's hyperparameter study

3 groups of plots are shown, one for each hash size: 96, 128, 192 bits. Results for 256 bits are presented in the main paper. With one hyperparameter value fixed, we compare:

- the maximum performance of ULA-CODE (max ULA-CODE)
- The average performance of ULA-CODE (avg ULA-CODE)
- LA-CODE's performance

Each row corresponds to one of the hyperparameters:  $\gamma, \theta, K_{bs}$ .

Each column corresponds to a test set: Bypass40, Cholec80, CEV64.

Each color corresponds to a level of observation: 1/3, 2/3, full video clip

96b

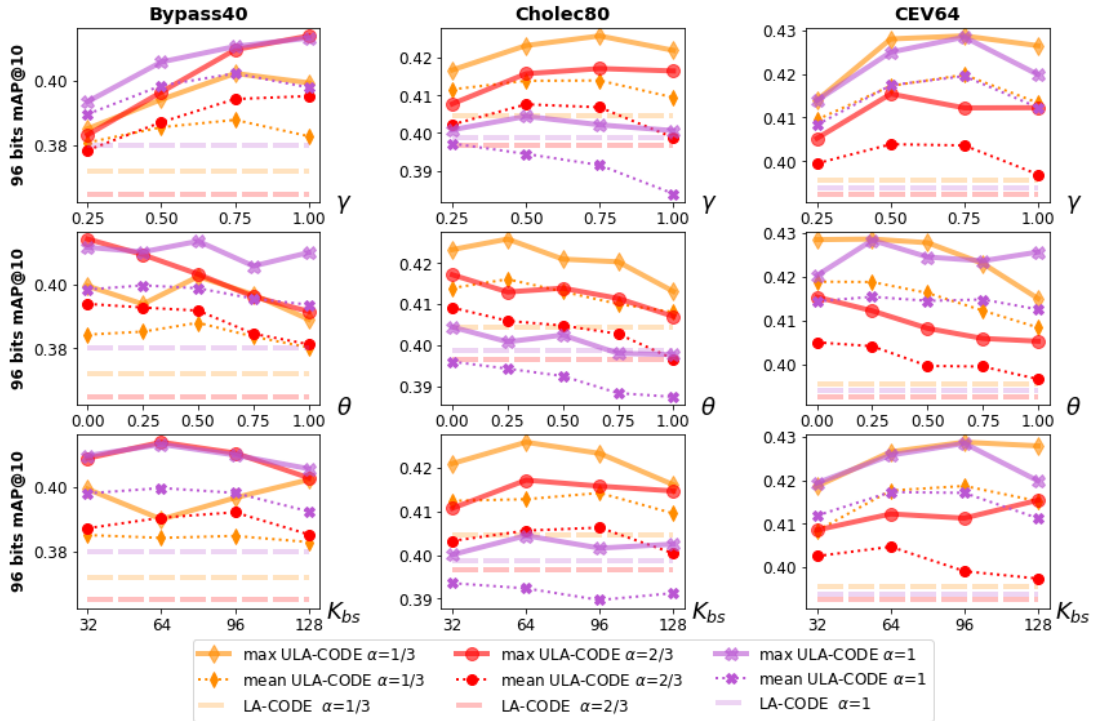

Figure 3: Hyperparameter study, 96 bit hashes

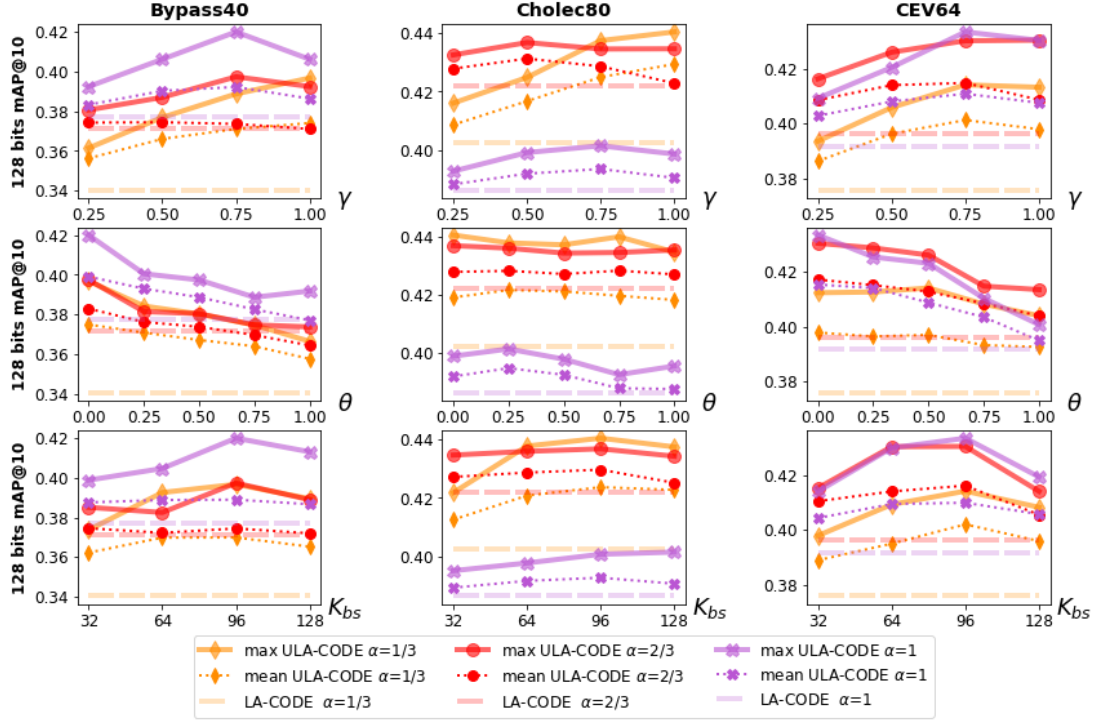

Figure 4: Hyperparameter study, 128 bit hashes

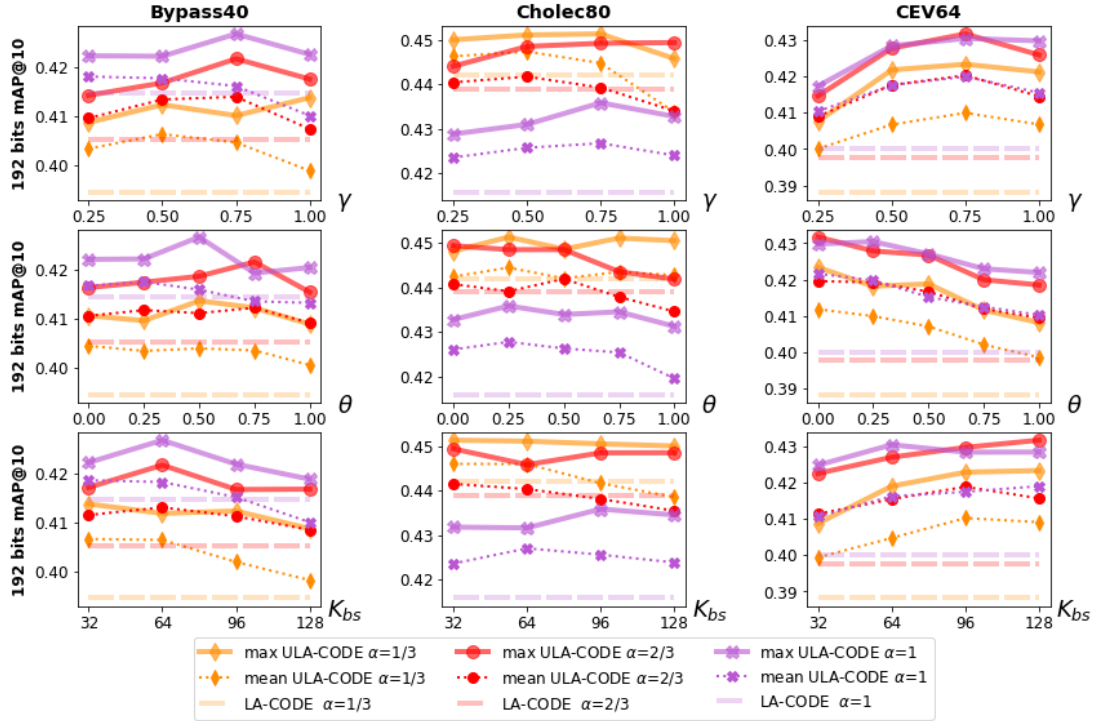

Figure 5: Hyperparameter study, 192 bit hashes

## C - Uncertainty pattern compression lower bound proof

As stated in Section 3.6, the position of exactly  $k$  uncertain bits in a  $2n$ -bit array can be flagged using **strictly** fewer than  $2n$  bits. Doing so saves  $d - \log_2 \binom{d}{k}$  bits, which has the following lower bound:

$$d - \log_2 \binom{d}{k} > \frac{1}{2} \log_2 \left( \frac{\pi \cdot d}{2} \right) \quad (1)$$

We will prove this inequality by bounding  $\log_2 \binom{d}{k}$  from above. The number of possible configurations for the position of  $k$  uncertain bits in an array of size  $2n$  is given by the binomial coefficient:

$$\binom{2n}{k} = \frac{(2n)!}{(2n-k)!(k!)} \quad (2)$$

The maximum is reached for the **central binomial coefficient**  $\binom{2n}{n} = \frac{(2n)!}{(n!)^2}$ . Indeed,  $\binom{2n}{k+1} = \frac{2n-k}{k+1} \binom{2n}{k} > \binom{2n}{k}$  for  $k < n$ . Therefore  $\binom{2n}{k}$  monotonously increases with  $k$  over the left side of  $n$ , and monotonously decreases over the right side due to  $\binom{2n}{k} = \binom{2n}{2n-k}$ , leaving  $\binom{2n}{n}$  as the maximum.

This means we have **at most**  $\binom{2n}{n}$  configurations to map to an  $m$ -bit array, requiring  $\log_2 \binom{2n}{n} \leq m$ . Bounding this term from above can be done via a result published by Dutton (Dutton and Brigham, 1986), which states:

$$\frac{1}{n+1} \binom{2n}{n} < \frac{4^n}{(n+1)\sqrt{\pi n}} \quad (3)$$

Or, equivalently:

$$\binom{2n}{n} < \frac{4^n}{\sqrt{\pi n}} \quad (4)$$

This is also apparent from the following series of inequalities (Elkies, 2013):

$$\binom{2n}{n} = \frac{4^n}{\pi} \int_{-\pi/2}^{\pi/2} \cos^{2n} x \, dx < \frac{4^n}{\pi} \int_{-\pi/2}^{\pi/2} e^{-nx^2} \, dx < \frac{4^n}{\pi} \int_{-\infty}^{\infty} e^{-nx^2} \, dx = \frac{4^n}{\sqrt{\pi n}}. \quad (5)$$

Note that it also is an asymptotic equivalent for  $\binom{2n}{n}$  (easily derived from Stirling's approximation  $n! \sim \sqrt{2\pi n} \left(\frac{n}{e}\right)^n$ ), making it an asymptotically tight upper bound.

Taking  $\log_2$  of the last term yields the desired lower bound:

$$2n - \log_2 \binom{2n}{n} > \frac{1}{2} \log_2 (\pi \cdot n) \quad (6)$$

The compression rate  $\log_2(\pi n)/4n$  tends to 0 as  $n$  tends towards  $+\infty$ ; however it should be noted that this is in the one worst case of  $k = n$ . Values closer to 0 or  $2n$  lead to much more favorable compression rates.

## References

- Dutton, Ronald D. and Robert C. Brigham (1986). “Computationally Efficient Bounds for the Catalan Numbers”. In: *European Journal of Combinatorics* 7.3, pp. 211–213. ISSN: 0195-6698. DOI: [https://doi.org/10.1016/S0195-6698\(86\)80024-5](https://doi.org/10.1016/S0195-6698(86)80024-5). URL: <https://www.sciencedirect.com/science/article/pii/S0195669886800245>.
- Elkies, Noam D. (2013). *Upper limit on the central binomial coefficient*. <https://mathoverflow.net/a/133752>.
